# Supplementary material for: (S)GD over Diagonal Linear Networks: Implicit Regularisation, Large Stepsizes and Edge of Stability
Source: arXiv:2302.08982 source file (2023-10-25)
Supplement: Supplementary file 1 [file concentration_old1.tex]

\section{Concentration of random matrices}\label{app:concentration}

\begin{lemma}\label{lemma:RIP}
Assuming that the data is from $\mathcal{N}(0, \sigma^2 I_d)$, \cref{ass:RIP1} is satisfied probability $1-\cO\left(\frac{1}{d^2}\right)$.
\end{lemma}


\begin{lemma}\label{lem:concentration1}
Let $x_1,\ldots,x_n\in\R^d$ be \emph{i.i.d.}~random variables of law $\cN(0,I_d)$. Let  $H=\frac{1}{n}\sum_{i=1}^nx_ix_i^\top$.
There exists $C_0,C_1>0$ such that if $\lambda$ is a non-null eigenvalue of $H$,
\begin{equation*}
    \P\left( |\lambda- \frac{d}{n}|\geq \frac{d}{2n}\right)\leq e^{-C_0d + C_1 n}\,.
\end{equation*}
\end{lemma}

\begin{lemma}\label{lem:concentration2}
Let $x_1,\ldots,x_n\in\R^d$ be \emph{i.i.d.}~random variables of law $\cN(\mu\one,\sigma^2I_d)$. Let  $H=\frac{1}{n}\sum_{i=1}^nx_ix_i^\top$ and $\tilde H=\frac{1}{n}\sum_{i=1}^n\NRM{x_i}^2 x_ix_i^\top$.
There exist numerical constants $C_2,C_3>0$ such that
    \begin{equation*}
        \P \Big( C_2\big(\mu^2+\sigma^2)d H \preceq  \tilde H \preceq  C_3\big(\mu^2+\sigma^2)d H\Big)\geq 1- 2ne^{-d/16}\,.
    \end{equation*}
\end{lemma}

\begin{lemma}\label{lem:concentration3}
Let $x_1,\ldots,x_n\in\R^d$ be \emph{i.i.d.}~random variables of law $\cN(0,I_d)$. Let  $H=\frac{1}{n}\sum_{i=1}^nx_ix_i^\top$ and for $1\leq b\leq n$ let $\tilde H_b=\E_\cB\left[\left(\frac{1}{b}\sum_{i\in\cB}x_ix_i^\top\right)^2\right]$ where $\cB\subset[n]$ is sampled uniformly at random in $\set{\cB\subset[n]\,\text{s.t.}\,|\cB|=b}$.
Then, there exist numerical constants $C_2',C_3'>0$ such that
    \begin{equation*}
        \P \Big(\frac{d}{b} C_2' H \preceq  \tilde H_b \preceq \frac{d}{b} C_3' H\Big)\geq 1- 2ne^{-d/16}\,.
    \end{equation*}
\end{lemma}

\Snote{to check by Mathieu, but the following lemma seems reasonable}
\begin{lemma}\label{lem:concentration3bis}
Let $x_1,\ldots,x_n\in\R^d$ be \emph{i.i.d.}~random variables of law $\cN(\mu \one, \sigma^2 I_d)$ for some $\mu\in\R$. Let  $H=\frac{1}{n}\sum_{i=1}^nx_ix_i^\top$ and for $1\leq b\leq n$ let $\tilde H_b=\E_\cB\left[\left(\frac{1}{b}\sum_{i\in\cB}x_ix_i^\top\right)^2\right]$ where $\cB\subset[n]$ is sampled uniformly at random in $\set{\cB\subset[n]\,\text{s.t.}\,|\cB|=b}$.
Then, there exist numerical constants $C_2',C_3'>0$ such that
    \begin{equation*}
        \P \Big((\mu^2 + \frac{\sigma^2 d}{b}) C_2' H \preceq  \tilde H_b \preceq (\mu^2 +  \frac{\sigma^2 d}{b}) C_3' H\Big)\geq 1- 2ne^{-d/16}\,.
    \end{equation*}
\end{lemma}

\begin{lemma}\label{lem:concentration4}
Let $x_1,\ldots,x_n\in\R^d$ be \emph{i.i.d.}~random variables of law $\cN(0,I_d)$ and  $H=\frac{1}{n}\sum_{i=1}^nx_ix_i^\top$.
Then, denoting by $\cC$ the set of all $s$-sparse vector $\beta\in\R^d$ satisfying $\NRM{\beta}_2\leq 1$, there exist $C_4,C_5>0$ such that for any $\eps>0$, if $n\geq C_4s\ln(d)\eps^{-2}$,
    \begin{equation*}
        \P\left(\sup_{\beta\in\cS}\NRM{H\beta-\beta}_\infty \geq \eps\right)\leq e^{-C_5 n}\,.
    \end{equation*}
\end{lemma}

\begin{proof}[Proof of Lemma~\ref{lem:concentration1}]
We start with the first point.
    Let $M=X^\top X\in\R^{n\times n}$ where $X=\frac{1}{n}(x_1,\ldots,x_n)\in\R^{d\times n}$. Since $H=XX^\top$, the eigenvalues of $H$ and $M$ are the same, so we only need to study those of $M$.
    
    Let $u\in\R^n$ such that $\NRM{u}_2=1$. Since $M_{i,j}=\sum_{k=1}^dx_{ik}x_{jk}$, we have:
    \begin{align*}
        nu^\top M u &= \sum_{1\leq i,j\leq n} \sum_{k=1}^d u_iu_jx_{ik}x_{jk}\\
        &=\sum_{k=1}^d \langle u,x_{:,k}\rangle^2\,,
    \end{align*}
    where $x_{:,k}=(x_{ik})_{i\in[n]}\sim\cN(0,I_n)$. Thus, using $\NRM{u}_2=1$, we have:
    \begin{equation*}
        nu^\top M u = \sum_{k=1}^d z_k^2\,,
    \end{equation*}
    where $z_k$ are iid random variables of law $\cN(0,1)$.
    Hence, using subexponential concentration inequalities \cite{vershynin_2018},
    \begin{equation*}
        \P\big(|\frac{n}{d}u^\top M u - 1| \geq t\big)\leq 2\exp(-cdt^2)\,,
    \end{equation*}
    for some constant $c>0$ and $t\leq 1$.
    Thus, using an $\eps$-net (of size $(C/\eps)^n$, and for $\eps$ of order 1) of the sphere of $\R^n$, we obtain that, for any $t\leq 1$:
    \begin{align*}
        \P\big(\sup_{\NRM{u}=1} |\frac{n}{d}u^\top M u - 1| \geq t\big)&\leq 2\exp(-cdt^2)\times C^n\\
        & = 2\exp\big( -cdt^2 + n\ln(C)\big)\,.
    \end{align*}
    Taking $t=\frac{1}{2}$ concludes the proof.
    \end{proof}
    
    \begin{proof}[Proof of Lemma~\ref{lem:concentration2}]
    First, we write $x_i=\mu\one+\sigma z_i$, where $z_i\sim\cN(0,I)$, leading to:
\begin{align*}
    \frac{1}{n}\sum_{i\in[n]}\NRM{x_i}_2^2 x_ix_i^\top &=\frac{1}{n}\sum_{i\in[n]}\big(\sigma^2\NRM{z_i}_2^2 + d\mu^2 + 2\sigma\mu\langle\one,z_i\rangle\big)  x_ix_i^\top 
\end{align*}
    We use concentration of $\chi_d^2$ random variables around $d$:
    \begin{equation*}
        \P(\chi^2_d>d + 2t+ 2\sqrt{dt})\geq t)\leq e^{-t} \quad\text{and}\quad \P(\chi^2_d>d  - 2\sqrt{dt})\leq t)\leq e^{-t}\,,
    \end{equation*}
    so that for all $i\in[n]$,
    \begin{equation*}
        \P(\NRM{z_i}_2^2\notin[d  - 2\sqrt{dt},d + 2t+ 2\sqrt{dt}] )\leq 2e^{-t}\,.
    \end{equation*}
    Thus,
    \begin{equation*}
        \P(\forall i\in[n], \,\NRM{z_i}_2^2\in[d  - 2\sqrt{dt},d + 2t+ 2\sqrt{dt}] ) \geq 1-2ne^{-t}\,.
    \end{equation*}
    Taking $t=d/16$, 
    \begin{equation*}
        \P(\forall i\in[n], \,\NRM{z_i}_2^2\in[\frac{d}{2},13d/8] ) \geq 1-2ne^{-d/16}\,.
    \end{equation*}
    Then, for all $i$, $\langle \one,z_i\rangle$ is of law $\cN(0,d)$, so that $\P(|\langle \one,z_i\rangle|\geq t)\leq2e^{-t^2/(2d)} $ and
    \begin{equation*}
        \P\big(\forall i\in[n],\,|\langle \one,z_i\rangle|\geq t\big)\leq 2ne^{-\frac{t^2}{2d}}\,.
    \end{equation*}
    Taking $t=\sqrt{2}d^{3/4}$,
    \begin{equation*}
                \P\big(\forall i\in[n],\,|\langle \one,z_i\rangle|\geq d^{3/4}\big)\leq 2ne^{-d^{1/2}}\,.
    \end{equation*}
    Thus, with probability $1-2n(e^{-d/16}+e^{-\sqrt{d}}$, we have $\forall i\in[n],\,|\langle \one,z_i\rangle|\geq d^{3/4}$ and $\NRM{z_i}_2^2\in[\frac{d}{2},13d/8]$, so that
    \begin{equation*}
        \big(\frac{d}{2}\sigma^2 + d\mu^2 -2\mu\sigma d^{3/4}\big) H\preceq \tilde H \preceq \big(\frac{13d}{8}\sigma^2 + d\mu^2 +2\mu\sigma d^{3/4}\big) H\,,
    \end{equation*}
    leading to the desired result.
\end{proof}

\begin{proof}[Proof of Lemma~\ref{lem:concentration3}]
We have:
\begin{align*}
    \tilde H_b&= \esp{\frac{1}{b^2}\sum_{i,j\in\cB}\langle x_i,x_j\rangle x_ix_j^\top}\\
    &= \esp{\frac{1}{b^2}\sum_{i\in\cB}\NRM{x_i}_2^2 x_ix_i^\top + \frac{1}{b^2}\sum_{i,j\in\cB,\,i\ne j}\langle x_i,x_j\rangle x_ix_j^\top}\\
    &=\frac{1}{b^2}\sum_{i\in[n]}\P(i\in\cB) \NRM{x_i}_2^2 x_ix_i^\top + \frac{1}{b^2} \sum_{i\ne j} \P(i,j\in\cB) \langle x_i,x_j\rangle x_ix_j^\top\,.
\end{align*}
Then, since $\P(i\in\cB)=\frac{b}{n}$ and $\P(i,j\in\cB)=\frac{b(b-1)}{n(n-1)}$ for $i\ne j$, we get that:
\begin{equation*}
    \tilde H_b=\frac{1}{bn}\sum_{i\in[n]}\NRM{x_i}_2^2 x_ix_i^\top + \frac{(b-1)}{bn(n-1)} \sum_{i\ne j} \langle x_i,x_j\rangle x_ix_j^\top\,.
\end{equation*}
Using Lemma~\ref{lem:concentration2}, the first term satisfies:
\begin{equation*}
    \P \Big( \frac{d}{b} C_2 H \preceq  \frac{1}{bn}\sum_{i\in[n]}\NRM{x_i}_2^2 x_ix_i^\top \preceq  \frac{d}{b} C_3 H\Big)\geq 1- 2ne^{-d/16}\,.
\end{equation*}
We now show that the second term is of order $\sqrt{d}H$.
For $i\ne j$, $\langle x_i,x_j\rangle=\sum_{k=1}^d x_{ik}x_{jk}=\sum_{k=1}^dz_k$ where $z_k=x_{ik}x_{jk}$ satisfes $\E z_k=0$, $\E z_k^2=1$ and $\P(z_k\geq t)\leq 2\P(|x_{ik}|\geq \sqrt{t})\leq 4 e^{-t/2}$.
Hence, $z_k$ is a centered subexponential random variables. Using concentration of  subexponential random variables \cite{vershynin_2018}, for $t\leq 1$,
\begin{equation*}
    \P\left(\frac{1}{d}| \langle x_i,x_j\rangle | \geq t\right)\leq 2e^{-cdt^2}\,.
\end{equation*}
Thus, 
\begin{equation*}
    \P\left(\forall i\ne j,\,\frac{1}{d}| \langle x_i,x_j\rangle | \leq t\right) \geq 1-n(n-1)e^{-cdt^2}\,.
\end{equation*}
Then, taking $t=d^{-1/2}4\ln(n)/c$, we have:
\begin{equation*}
        \P\left(\forall i\ne j,\,\frac{1}{d}| \langle x_i,x_j\rangle | \leq \frac{4\ln(n)}{c\sqrt{d}}\right) \geq 1-\frac{1}{n^2}\,.
\end{equation*}
Going back to our second term,
\begin{align*}
    \frac{(b-1)}{bn(n-1)} \sum_{i\ne j} \langle x_i,x_j\rangle x_ix_j^\top &= \frac{(b-1)}{bn(n-1)} \sum_{i<j} \langle x_i,x_j\rangle \big(x_ix_j^\top+x_jx_i^\top\big)\\
    &\preceq  \frac{(b-1)}{bn(n-1)} \sum_{i<j} \big|\langle x_i,x_j\rangle\big| \big(x_ix_i^\top+x_jx_j^\top\big)\,,
\end{align*}
where we used $x_ix_j^\top+x_jx_i^\top\preceq x_ix_i^\top+x_jx_j^\top$. Thus,
\begin{align*}
    \frac{(b-1)}{bn(n-1)} \sum_{i\ne j} \langle x_i,x_j\rangle x_ix_j^\top&\preceq \sup_{i\ne j}|\langle x_i,x_j\rangle| \times \frac{(b-1)}{bn(n-1)} \sum_{i<j} \big(x_ix_i^\top+x_jx_j^\top\big)\\
    &=\sup_{i\ne j}|\langle x_i,x_j\rangle| \times \frac{b-1}{b} \frac{1}{n-1} \sum_{i=1}^n x_ix_i^\top\\
    &=\sup_{i\ne j}|\langle x_i,x_j\rangle| \times \frac{b-1}{b} \frac{n}{n-1} H\,.
\end{align*}
Similarly, we have
\begin{equation*}
    \frac{(b-1)}{bn(n-1)} \sum_{i\ne j} \langle x_i,x_j\rangle x_ix_j^\top\succeq -\sup_{i\ne j}|\langle x_i,x_j\rangle| \times \frac{b-1}{b} \frac{n}{n-1} H\,.
\end{equation*}
Hence, with probability $1-1/n^2$,
\begin{equation*}
    - \frac{4\ln(n)}{c\sqrt{d}} \times \frac{b-1}{b} \frac{n}{n-1} H\preceq \frac{(b-1)}{bn(n-1)} \sum_{i\ne j} \langle x_i,x_j\rangle x_ix_j^\top \preceq  \frac{4\ln(n)}{c\sqrt{d}} \times \frac{b-1}{b} \frac{n}{n-1} H\,.
\end{equation*}
Wrapping things up, with probability $1-1/n^2-2ne^{-d/16}$,
\begin{equation*}
        \left(- \frac{4\ln(n)}{c\sqrt{d}}  \frac{b-1}{b} \frac{n}{n-1} + C_2\frac{d}{b}\right)\times H\preceq \tilde H_b \preceq  \left(\frac{4\ln(n)}{c\sqrt{d}}  \frac{b-1}{b} \frac{n}{n-1} + C_3\frac{d}{b}\right)\times H\,.
\end{equation*}
Thus, provided that $\frac{4\ln(n)}{c\sqrt{d}}  \leq \frac{C_2d}{2b}$ and $d\geq 48\ln(n)$, we have with probability $1-3/n^2$:
\begin{equation*}
     C_2'\frac{d}{b}\times H\preceq \tilde H_b \preceq   C_3'\frac{d}{b}\times H\,.
\end{equation*}
\end{proof}

\begin{proof}[Proof of Lemma~\ref{lem:concentration3bis}]
We have:
\begin{align*}
    \tilde H_b&= \esp{\frac{1}{b^2}\sum_{i,j\in\cB}\langle x_i,x_j\rangle x_ix_j^\top}\\
    &= \esp{\frac{1}{b^2}\sum_{i\in\cB}\NRM{x_i}_2^2 x_ix_i^\top + \frac{1}{b^2}\sum_{i,j\in\cB,\,i\ne j}\langle x_i,x_j\rangle x_ix_j^\top}\\
    &=\frac{1}{b^2}\sum_{i\in[n]}\P(i\in\cB) \NRM{x_i}_2^2 x_ix_i^\top + \frac{1}{b^2} \sum_{i\ne j} \P(i,j\in\cB) \langle x_i,x_j\rangle x_ix_j^\top\,.
\end{align*}
Then, since $\P(i\in\cB)=\frac{b}{n}$ and $\P(i,j\in\cB)=\frac{b(b-1)}{n(n-1)}$ for $i\ne j$, we get that:
\begin{equation*}
    \tilde H_b=\frac{1}{bn}\sum_{i\in[n]}\NRM{x_i}_2^2 x_ix_i^\top + \frac{(b-1)}{bn(n-1)} \sum_{i\ne j} \langle x_i,x_j\rangle x_ix_j^\top\,.
\end{equation*}
Using Lemma~\ref{lem:concentration2}, the first term satisfies:
\begin{equation*}
    \P \Big( \frac{d(\mu^2+\sigma^2)}{b} C_2 H \preceq  \frac{1}{bn}\sum_{i\in[n]}\NRM{x_i}_2^2 x_ix_i^\top \preceq  \frac{d(\mu^2+\sigma^2)}{b} C_3 H\Big)\geq 1- 2ne^{-d/16}\,.
\end{equation*}
We now show that the second term is of smaller order.
Writing $x_i=\mu\one+\sigma z_i$ where $z_i\sim\cN(0,I_d)$, we have:
\begin{align*}
    \frac{(b-1)}{bn(n-1)} \sum_{i\ne j} \langle x_i,x_j\rangle x_ix_j^\top=\frac{(b-1)}{bn(n-1)} \sum_{i\ne j} \langle x_i,x_j\rangle x_ix_j^\top
\end{align*}

For $i\ne j$, $\langle x_i,x_j\rangle=\sum_{k=1}^d x_{ik}x_{jk}=\sum_{k=1}^da_k$ where $a_k=x_{ik}x_{jk}$ satisfies $\E a_k=0$, $\E a_k^2=1$ and $\P(a_k\geq t)\leq 2\P(|x_{ik}|\geq \sqrt{t})\leq 4 e^{-t/2}$.
Hence, $a_k$ is a centered subexponential random variables. Using concentration of  subexponential random variables \cite{vershynin_2018}, for $t\leq 1$,
\begin{equation*}
    \P\left(\frac{1}{d}| \langle x_i,x_j\rangle | \geq t\right)\leq 2e^{-cdt^2}\,.
\end{equation*}
Thus, 
\begin{equation*}
    \P\left(\forall i\ne j,\,\frac{1}{d}| \langle x_i,x_j\rangle | \leq t\right) \geq 1-n(n-1)e^{-cdt^2}\,.
\end{equation*}
Then, taking $t=d^{-1/2}4\ln(n)/c$, we have:
\begin{equation*}
        \P\left(\forall i\ne j,\,\frac{1}{d}| \langle x_i,x_j\rangle | \leq \frac{4\ln(n)}{c\sqrt{d}}\right) \geq 1-\frac{1}{n^2}\,.
\end{equation*}
Going back to our second term,
\begin{align*}
    \frac{(b-1)}{bn(n-1)} \sum_{i\ne j} \langle x_i,x_j\rangle x_ix_j^\top &= \frac{(b-1)}{bn(n-1)} \sum_{i<j} \langle x_i,x_j\rangle \big(x_ix_j^\top+x_jx_i^\top\big)\\
    &\preceq  \frac{(b-1)}{bn(n-1)} \sum_{i<j} \big|\langle x_i,x_j\rangle\big| \big(x_ix_i^\top+x_jx_j^\top\big)\,,
\end{align*}
where we used $x_ix_j^\top+x_jx_i^\top\preceq x_ix_i^\top+x_jx_j^\top$. Thus,
\begin{align*}
    \frac{(b-1)}{bn(n-1)} \sum_{i\ne j} \langle x_i,x_j\rangle x_ix_j^\top&\preceq \sup_{i\ne j}|\langle x_i,x_j\rangle| \times \frac{(b-1)}{bn(n-1)} \sum_{i<j} \big(x_ix_i^\top+x_jx_j^\top\big)\\
    &=\sup_{i\ne j}|\langle x_i,x_j\rangle| \times \frac{b-1}{b} \frac{1}{n-1} \sum_{i=1}^n x_ix_i^\top\\
    &=\sup_{i\ne j}|\langle x_i,x_j\rangle| \times \frac{b-1}{b} \frac{n}{n-1} H\,.
\end{align*}
Similarly, we have
\begin{equation*}
    \frac{(b-1)}{bn(n-1)} \sum_{i\ne j} \langle x_i,x_j\rangle x_ix_j^\top\succeq -\sup_{i\ne j}|\langle x_i,x_j\rangle| \times \frac{b-1}{b} \frac{n}{n-1} H\,.
\end{equation*}
Hence, with probability $1-1/n^2$,
\begin{equation*}
    - \frac{4\ln(n)}{c\sqrt{d}} \times \frac{b-1}{b} \frac{n}{n-1} H\preceq \frac{(b-1)}{bn(n-1)} \sum_{i\ne j} \langle x_i,x_j\rangle x_ix_j^\top \preceq  \frac{4\ln(n)}{c\sqrt{d}} \times \frac{b-1}{b} \frac{n}{n-1} H\,.
\end{equation*}
Wrapping things up, with probability $1-1/n^2-2ne^{-d/16}$,
\begin{equation*}
        \left(- \frac{4\ln(n)}{c\sqrt{d}}  \frac{b-1}{b} \frac{n}{n-1} + C_2\frac{d}{b}\right)\times H\preceq \tilde H_b \preceq  \left(\frac{4\ln(n)}{c\sqrt{d}}  \frac{b-1}{b} \frac{n}{n-1} + C_3\frac{d}{b}\right)\times H\,.
\end{equation*}
Thus, provided that $\frac{4\ln(n)}{c\sqrt{d}}  \leq \frac{C_2d}{2b}$ and $d\geq 48\ln(n)$, we have with probability $1-3/n^2$:
\begin{equation*}
     C_2'\frac{d}{b}\times H\preceq \tilde H_b \preceq   C_3'\frac{d}{b}\times H\,.
\end{equation*}
\end{proof}

\begin{proof}[Proof of Lemma~\ref{lem:concentration4}]
For $j\in[d]$, we have:
\begin{align*}
    (H\beta)_j &= \frac{1}{n}\sum_{i=1}^n x_{ij}\langle x_i,\beta\rangle\\
    &=\frac{1}{n}\sum_{i=1}^n\sum_{j'=1}^d x_{ij}x_{ij'}\beta_{j'}\\
    &=\frac{1}{n}\sum_{i=1}^n x_{ij}^2\beta_{j}+\frac{1}{n}\sum_{i=1}^n\sum_{j'\ne j} x_{ij}x_{ij'}\beta_{j'} \\
    &=\frac{\beta_j}{n}\sum_{i=1}^n x_{ij}^2+\frac{1}{n}\sum_{i=1}^nx_{ij}\sum_{j'\ne j} x_{ij'}\beta_{j'} \,.
\end{align*}
We thus notice that $\esp{H\beta}=\beta$, and 
\begin{equation*}
    (H\beta)_j= \beta_j + \frac{\beta_j}{n}\sum_{i=1}^n (x_{ij}^2-1)+\frac{1}{n}\sum_{i=1}^nz_i\,,
\end{equation*}
where $z_i=x_{ij}\sum_{j'\ne j} x_{ij'}\beta_{j'}$, and $\sum_{j'\ne j} x_{ij'}\beta_{j'}\sim\cN(0,\NRM{\beta}^2-\beta_j^2)$ and $\NRM{\beta}^2-\beta_j^2\leq 1$. Hence, $z_j+x_{ij}^2-1$ is a centered subexponential random variables (with a subexponential parameter of order 1). Thus, for $t\leq 1$:
\begin{equation*}
    \P\left(\left| \frac{\beta_j}{n}\sum_{i=1}^n (x_{ij}^2-1)+\frac{1}{n}\sum_{i=1}^nz_i \right|\geq t\right)\leq 2e^{-cnt^2}\,.
\end{equation*}
Hence, using an $\eps$-net of $\cC=\set{\beta\in\R^d:\, \NRM{\beta}_2\leq 1\,,\NRM{\beta}_0}$ (of cardinality less than $d^s\times(C/\eps)^s$, and for $\eps$ of order 1), we have:
\begin{equation*}
    \P\left(\sup_{\beta\in\cC,\,j\in[d]}\left| (H\beta)_j-\beta_j \right|\geq t\right)\leq d\times d^s(C/\eps)^s\times 2e^{-cnt^2}=\exp\left(-c\ln(2)nt^2 + (s+1)\ln(d) + s \ln(C/\eps)\right)\,.
\end{equation*}
Consequently, for $t=\eps$ and if $n\geq C_4 s\ln(d)/\eps^2$, we have:
\begin{equation*}
    \P\left(\sup_{\beta\in\cC,\,j\in[d]}\left| (H\beta)_j-\beta_j \right|\geq t\right)\leq\exp\left(-C_5nt^2 \right)\,.
\end{equation*}



\end{proof}

\mathieu{New version I wrote in the train that I think is correct.}

\begin{lemma}\label{lem:concentration3bis}
Let $x_1,\ldots,x_n\in\R^d$ be \emph{i.i.d.}~random variables of law $\cN(\mu \one, \sigma^2 I_d)$ for some $\mu\in\R$. Let  $H=\frac{1}{n}\sum_{i=1}^nx_ix_i^\top$ and for $1\leq b\leq n$ let $\tilde H_b=\E_\cB\left[\left(\frac{1}{b}\sum_{i\in\cB}x_ix_i^\top\right)^2\right]$ where $\cB\subset[n]$ is sampled uniformly at random in $\set{\cB\subset[n]\,\text{s.t.}\,|\cB|=b}$.
With probability $1-2ne^{-d/16}-3/n^2$, we have, for some numerical constants $c_1,c_2,c_3,C>0$:
\begin{equation*}
    \left( c_1\frac{d(\mu^2+\sigma^2)}{b} - c_2\frac{(\sigma^2+\mu^2)\ln(n)}{\sqrt{d}} - c_3\frac{\mu^2 d}{n}\right)H \preceq \tilde H_b \preceq C\left( \frac{d(\mu^2+\sigma^2)}{b} + \frac{(\sigma^2+\mu^2)\ln(n)}{\sqrt{d}} + \mu^2 d\right)
\end{equation*}
\end{lemma}


\begin{proof}[Proof of Lemma~\ref{lem:concentration3bis}]
We have:
\begin{align*}
    \tilde H_b&= \esp{\frac{1}{b^2}\sum_{i,j\in\cB}\langle x_i,x_j\rangle x_ix_j^\top}\\
    &= \esp{\frac{1}{b^2}\sum_{i\in\cB}\NRM{x_i}_2^2 x_ix_i^\top + \frac{1}{b^2}\sum_{i,j\in\cB,\,i\ne j}\langle x_i,x_j\rangle x_ix_j^\top}\\
    &=\frac{1}{b^2}\sum_{i\in[n]}\P(i\in\cB) \NRM{x_i}_2^2 x_ix_i^\top + \frac{1}{b^2} \sum_{i\ne j} \P(i,j\in\cB) \langle x_i,x_j\rangle x_ix_j^\top\,.
\end{align*}
Then, since $\P(i\in\cB)=\frac{b}{n}$ and $\P(i,j\in\cB)=\frac{b(b-1)}{n(n-1)}$ for $i\ne j$, we get that:
\begin{equation*}
    \tilde H_b=\frac{1}{bn}\sum_{i\in[n]}\NRM{x_i}_2^2 x_ix_i^\top + \frac{(b-1)}{bn(n-1)} \sum_{i\ne j} \langle x_i,x_j\rangle x_ix_j^\top\,.
\end{equation*}
Using Lemma~\ref{lem:concentration2}, the first term satisfies:
\begin{equation*}
    \P \Big( \frac{d(\mu^2+\sigma^2)}{b} C_2 H \preceq  \frac{1}{bn}\sum_{i\in[n]}\NRM{x_i}_2^2 x_ix_i^\top \preceq  \frac{d(\mu^2+\sigma^2)}{b} C_3 H\Big)\geq 1- 2ne^{-d/16}\,.
\end{equation*}
We now show that the second term is of smaller order.
Writing $x_i=\mu\one+\sigma z_i$ where $z_i\sim\cN(0,I_d)$, we have:
\begin{align*}
    \frac{(b-1)}{bn(n-1)} \sum_{i\ne j} \langle x_i,x_j\rangle x_ix_j^\top&=\frac{(b-1)}{bn(n-1)} \sum_{i\ne j}\big( \sigma^2\langle z_i,z_j\rangle +\sigma\mu\langle\one,z_i+z_j\rangle +\mu^2 d \big)x_ix_j^\top\\
    &= \frac{(b-1)}{bn(n-1)} \sum_{i\ne j}\big( \sigma^2\langle z_i,z_j\rangle +\sigma\mu\langle\one,z_i+z_j\rangle\big)x_ix_j^\top +\frac{(b-1)}{bn(n-1)} \mu^2 d \sum_{i\ne j}x_ix_j^\top
\end{align*}
For $i\ne j$, $\langle z_i,z_j\rangle=\sum_{k=1}^d z_{ik}z_{jk}=\sum_{k=1}^da_k$ where $a_k=z_{ik}z_{jk}$ satisfies $\E a_k=0$, $\E a_k^2=1$ and $\P(a_k\geq t)\leq 2\P(|z_{ik}|\geq \sqrt{t})\leq 4 e^{-t/2}$.
Hence, $a_k$ is a centered subexponential random variables. Using concentration of  subexponential random variables \cite{vershynin_2018}, for $t\leq 1$,
\begin{equation*}
    \P\left(\frac{1}{d}| \langle x_i,x_j\rangle | \geq t\right)\leq 2e^{-cdt^2}\,.
\end{equation*}
Thus, 
\begin{equation*}
    \P\left(\forall i\ne j,\,\frac{1}{d}| \langle x_i,x_j\rangle | \leq t\right) \geq 1-n(n-1)e^{-cdt^2}\,.
\end{equation*}
Then, taking $t=d^{-1/2}4\ln(n)/c$, we have:
\begin{equation*}
        \P\left(\forall i\ne j,\,\frac{1}{d}| \langle x_i,x_j\rangle | \leq \frac{4\ln(n)}{c\sqrt{d}}\right) \geq 1-\frac{1}{n^2}\,.
\end{equation*}
For $i\in[n]$, $\langle \one , z_i\rangle\sim \cN(0,d)$ so that $\P(|\langle \one , z_i\rangle|\geq t)\leq 2e^{-t^2/(2d)}$, and
\begin{equation*}
    \P(\forall i\in[n],\,|\langle \one , z_i\rangle|\leq t)\geq 1-2ne^{-t^2/(2d)}=1-\frac{2}{n^2}\,,
\end{equation*}
for $t=3\sqrt{d}\ln(n)$. Hence, with probability $1-3/n^2$, for all $i\ne j$ we have $|\sigma^2\langle z_i,z_j\rangle +\sigma\mu\langle\one,z_i+z_j\rangle|\leq (\sigma^2+\sigma\mu)C\ln(n)/\sqrt{d}$.

Now,
\begin{align*}
    \frac{(b-1)}{bn(n-1)} \sum_{i\ne j} \big( \sigma^2\langle z_i,z_j\rangle +\sigma\mu\langle\one,z_i+z_j\rangle\big) x_ix_j^\top &=  \frac{(b-1)}{bn(n-1)} \sum_{i< j} \big( \sigma^2\langle z_i,z_j\rangle +\sigma\mu\langle\one,z_i+z_j\rangle\big) (x_ix_j^\top +x_jx_i^\top) \\
    &\preceq  \frac{(b-1)}{bn(n-1)} \sum_{i<j} \big| \sigma^2\langle z_i,z_j\rangle +\sigma\mu\langle\one,z_i+z_j\rangle\big)| \big(x_ix_i^\top+x_jx_j^\top\big)\,,
\end{align*}
where we used $x_ix_j^\top+x_jx_i^\top\preceq x_ix_i^\top+x_jx_j^\top$. Thus,
\begin{align*}
    \frac{(b-1)}{bn(n-1)} \sum_{i\ne j} \big( \sigma^2\langle z_i,z_j\rangle +\sigma\mu\langle\one,z_i+z_j\rangle\big) x_ix_j^\top&\preceq \sup_{i\ne j}\big| \sigma^2\langle z_i,z_j\rangle +\sigma\mu\langle\one,z_i+z_j\rangle\big)| \times \frac{(b-1)}{bn(n-1)} \sum_{i<j} \big(x_ix_i^\top+x_jx_j^\top\big)\\
    &=\sup_{i\ne j}\big| \sigma^2\langle z_i,z_j\rangle +\sigma\mu\langle\one,z_i+z_j\rangle\big| \times \frac{b-1}{b} \frac{1}{n-1} \sum_{i=1}^n x_ix_i^\top\\
    &=\sup_{i\ne j}\big| \sigma^2\langle z_i,z_j\rangle +\sigma\mu\langle\one,z_i+z_j\rangle\big| \times \frac{b-1}{b} \frac{n}{n-1} H\,.
\end{align*}
Similarly, we have
\begin{equation*}
    \frac{(b-1)}{bn(n-1)} \sum_{i\ne j} \big( \sigma^2\langle z_i,z_j\rangle +\sigma\mu\langle\one,z_i+z_j\rangle\big) x_ix_j^\top\succeq -\sup_{i\ne j}\big| \sigma^2\langle z_i,z_j\rangle +\sigma\mu\langle\one,z_i+z_j\rangle\big)| \times \frac{b-1}{b} \frac{n}{n-1} H\,.
\end{equation*}
Hence, with probability $1-3/n^2$,
\begin{equation*}
    - \frac{(\sigma^2+\sigma\mu)C\ln(n)}{\sqrt{d}} \times \frac{b-1}{b} \frac{n}{n-1} H\preceq \frac{(b-1)}{bn(n-1)} \sum_{i\ne j} \big( \sigma^2\langle z_i,z_j\rangle +\sigma\mu\langle\one,z_i+z_j\rangle\big) x_ix_j^\top \preceq  \frac{(\sigma^2+\sigma\mu)C\ln(n)}{\sqrt{d}}  \times \frac{b-1}{b} \frac{n}{n-1} H\,.
\end{equation*}
We thus have shown that this term (the one in the middle of the above inequality) is of smaller order.

We are hence left with $\frac{(b-1)}{bn(n-1)} \mu^2 d\sum_{i\ne j}x_i x_j^\top$.
Denoting $\bar x=\frac{1}{n}\sum_i x_i$, we have $\frac{1}{n^2}\sum_{i\ne j}x_ix_j^\top = \frac{1}{n^2}\sum_{i, j}x_ix_j^\top  -\frac{1}{n^2}\sum_{i}x_ix_i^\top $, so that:
\begin{equation*}
    \frac{(b-1)}{bn(n-1)} \mu^2 d\sum_{i\ne j}x_i x_j^\top = \frac{(b-1)n}{b(n-1)} \left( \bar x\bar x^\top - \frac{1}{n}H \right)\,.
\end{equation*}
Noting that we have $H= \frac{1}{n}\sum_i \bar x_i x_i^\top = \frac{1}{n^2}\sum_{i<j}x_ix_i^\top + x_jx_j^\top\succeq \frac{1}{n^2}\sum_{i<j} x_i x_j^\top+x_jx_i^\top = \bar x\bar x^\top $ using $x_ix_i^\top + x_jx_j^\top \succeq x_ix_j^\top + x_jx_i^\top$. Thus, $H\succeq \bar x\bar x^\top\succeq 0$, and:
\begin{equation*}
    -\frac{(b-1)n}{b(n-1)} \mu^2 d \frac{1}{n} H\preceq \frac{(b-1)}{bn(n-1)} \mu^2 d\sum_{i\ne j}x_i x_j^\top \preceq \frac{(b-1)n}{b(n-1)} \mu^2 d (1-1/n) H\,.
\end{equation*}

We are now able to wrap everything together.
With probability $1-2ne^{-d/16}-3/n^2$, we have, for some numerical constants $c_1,c_2,c_3,C>0$:
\begin{equation*}
    \left( c_1\frac{d(\mu^2+\sigma^2)}{b} - c_2\frac{(\sigma^2+\mu^2)\ln(n)}{\sqrt{d}} - c_3\frac{\mu^2 d}{n}\right)H \preceq \tilde H_b \preceq C\left( \frac{d(\mu^2+\sigma^2)}{b} + \frac{(\sigma^2+\mu^2)\ln(n)}{\sqrt{d}} + \mu^2 d\right)
\end{equation*}

\end{proof}


\begin{lemma}\label{lem:concentration1bis}
Let $x_1,\ldots,x_n\in\R^d$ be \emph{i.i.d.}~random variables of law $\cN(\mu,\sigma^2I_d)$. Let  $H=\frac{1}{n}\sum_{i=1}^nx_ix_i^\top$.
There exists $C_0,C_1>0$ such that with probability $1-e^{-C_0d + C_1 n}$, $H$ is of rank $n$ and its non-null eigenvalues $\lambda_1\geq \dots\geq\lambda_n>0$ satisfy
\begin{equation*}
    C_1d\left(\mu^2 + \frac{\sigma^2}{n}\right) \leq\lambda_1 \leq C_2d\left(\mu^2 + \frac{\sigma^2}{n}\right)\,,\quad\text{and}\quad C_1d\frac{\mu^2+\sigma^2}{n}\leq \lambda_i\leq C_2d\frac{\mu^2+\sigma^2}{n}\quad \forall i\in\set{2,\ldots,n}\,.
\end{equation*}
\end{lemma}

\begin{proof}[Proof of Lemma~\ref{lem:concentration1bis}]
We write $x_i=\mu\one+ \sigma z_i$ for $z_i\sim\cN(0,1)$.
    Let $M=X^\top X\in\R^{n\times n}$ where $X=\frac{1}{n}(x_1,\ldots,x_n)\in\R^{d\times n}$. Since $H=XX^\top$, the eigenvalues of $H$ and $M$ are the same, so we only need to study those of $M$.
    
    Let $u\in\R^n$ such that $\NRM{u}_2=1$. Since $M_{i,j}=\frac{1}{n}\sum_{k=1}^dx_{ik}x_{jk} = \frac{d}{n}\mu^2 + \frac{\sigma\mu}{n}\sum_{k=1}^dz_{ik}+z_{jk} + \frac{\sigma^2}{n}\sum_{k=1}^dz_{ik}z_{jk}  $, we have:
    \begin{align*}
        nu^\top M u &= \sum_{1\leq i,j\leq n} \sum_{k=1}^d u_iu_j(\sigma^2 z_{ik}z_{jk} + d\mu^2 + \sigma\mu (z_{ik}+z_{jk})\\
        &= d\mu^2\left(\sum_{i=1}^nu_i\right)^2+ \sigma^2 \sum_{k=1}^d \langle u,z_{:,k}\rangle^2 + 2\sigma\mu\sum_{i=1}^n u_i \sum_{k=1}^d\langle z_{:,k}, u\rangle\,,
    \end{align*}
    where $z_{:,k}=(z_{ik})_{i\in[n]}\sim\cN(0,I_n)$.
    
    We now bound all these three terms.
    The first one is the easiest to study since it is deterministic: for $u=\lambda\one/\sqrt{n}+ v$ where $v\top \one=0$, we have $d\mu^2\left(\sum_{i=1}^nu_i\right)^2= dn\mu^2\lambda^2$.
    
    Then, using $\NRM{u}_2=1$, we have:
    \begin{equation*}
        \sum_{k=1}^d \langle u,z_{:,k}\rangle^2=\sum_{k=1}^d a_k^2\,,
    \end{equation*}
    where $a_k$ are iid random variables of law $\cN(0,1)$.
    Hence, using subexponential concentration inequalities \cite{vershynin_2018},
    \begin{equation*}
        \P\big(|\frac{n}{d}\sum_{k=1}^d \langle u,z_{:,k}\rangle^2 - 1| \geq t\big)\leq 2\exp(-cdt^2)\,,
    \end{equation*}
    for some constant $c>0$ and $t\leq 1$.
    Thus, using an $\eps$-net (of size $(C/\eps)^n$, and for $\eps$ of order 1) of the sphere of $\R^n$, we obtain that, for any $t\leq 1$:
    \begin{align*}
        \P\big(\sup_{\NRM{u}=1} |\frac{n}{d}\sum_{k=1}^d \langle u,z_{:,k}\rangle^2 - 1| \geq t\big)&\leq 2\exp(-cdt^2)\times C^n\\
        & = 2\exp\big( -cdt^2 + n\ln(C)\big)\,.
    \end{align*}
    Taking $t=\frac{1}{2}$ we have $\frac{d}{2n}\leq \sum_{k=1}^d \langle u,z_{:,k}\rangle^2\leq \frac{3d}{2n}$ with probability $1-e^{-c_1 d + c_2 n}$.
    
    We now show that the third term $2\sigma\mu\sum_{i=1}^n u_i \sum_{k=1}^d\langle z_{:,k}, u\rangle$ is of smaller order.
    Using $\NRM{u}=1$, $\langle z_{:,k}, u\rangle\sim \cN(0,1)$, and by independence, $\sum_{k=1}^d\langle z_{:,k}, u\rangle\sim\cN(0,d)$, so that $\P(|\sum_{k=1}^d\langle z_{:,k}, u\rangle|\geq t)\leq 2e^{-t^2/(2d)}$.
    
    We are now able to prove our bounds on the eigenvalues of $M$.
    
    \mathieu{Conclude using $\lambda_1\leq \sup_u u^\top M u$ and $\lambda_1\geq u^\top M u$ for $u=\one/\sqrt{n}$.
    
    Then $\lambda_2\leq \sup_{u\in\R^d,\,\one\top u=0}u^\top M u$ and $\lambda_n\geq$ avec terme du milieu juste?}
    
    \end{proof}
